# Supplementary material for: Magnetic-field-induced reorientation in the SDW and the spin-stripe phases of the frustrated spin-1/2 chain compound $\beta$-TeVO$_4$
Source: arXiv:2007.00932 source file (2020-07-02)
Supplement: Supplementary file 1 [file betaTeVO4_SupplementMat.pdf]

# Supplementary material:
# Magnetic-field-induced reorientation in the SDW and the spin-stripe phases of the frustrated spin-$1/2$ chain compound $\beta$-TeVO$_4$

Mirta Herak,[1,*] Nikolina Novosel,[1] Martina Dragičević,[1] Thierry Guizouarn,[2] Olivier Cador,[2] Helmuth Berger,[3] Matej Pregelj,[4] Andrej Zorko,[4,5] and Denis Arčon[4,5]

[1] *Institute of Physics, Bijenička c. 46, HR-10000 Zagreb, Croatia*
[2] *Institut des Sciences Chimiques de Rennes UMR 6226, Université de Rennes 1, Campus de Beaulieu, 35042 Rennes, France*
[3] *Institut de Physique de la Matière Complexe, EPFL, CH-1015 Lausanne, Switzerland*
[4] *Jožef Stefan Institute, Jamova 39, 1000 Ljubljana, Slovenia*
[5] *Faculty of Mathematics and Physics, Jadranska 19, 1000 Ljubljana, Slovenia*

## LOW-FIELD TORQUE MEASUREMENT ($\mu_0 H \leq 1$ T)

In the context of spin reorientations presented in the main text, low magnetic field is the field which is not sufficient to induce spin reorientation, and for which, therefore, the measured curves can be described by Eqs. (1) in the main text. For $\beta$-TeVO$_4$ this is true for $\mu_0 H \leq 1$ T. Furthermore, in low magnetic field ($\mu_0 H < 1$ T) the phase diagram of $\beta$-TeVO$_4$ is isotropic - values of the transition temperatures $T_{N_1}$, $T_{N_2}$ and $T_{N_3}$ do not change when the magnetic field is applied along the $a$, $b$ or $c$ axis [1–3]. The fact that the low-field values correspond for these two phenomena (no spin reorientation and isotropy of the phase boundaries) is to be expected, since the driving mechanism for both phenomena are anisotropic exchange interactions. As the field increases, the phase diagram becomes anisotropic [1, 2].

The anisotropic magnetic phase diagram of $\beta$-TeVO$_4$ can be obtained from the measured angular dependencies of magnetic torque by plotting temperature- and field-dependence of torque for each sample position (angle of magnetic field with respect to crystal axes). In order to determine the phase boundaries, we first take a look at torque results obtained in low magnetic field.

In Fig. S1 and S2 we show angular dependence of torque measured in the $ac$ and $a^*b$ plane in $\mu_0 H = 0.2$ T and $\mu_0 H = 1$ T, respectively. Data for $\mu_0 H = 0.2$ T was used in previous publication which explored low-field magnetic anisotropy of the three ordered magnetic phases [4]. In low magnetic field the angular dependence of torque can be described by Eqs. (1a) and (1b) from the main text (solid black lines in Fig. S1 and S2). The temperature dependence of the phase $\theta_1$ in the $ac$ plane measured in $\mu_0 H = 0.2$ T is shown in the middle panel of Fig. S1. $\theta_1$ rotates temperature in the direction from $-c$ towards $a^*$ and stop when $\theta_1$ co-aligns with the angle of $\approx [1\,0\,\bar{1}]$ axis (middle panel of Fig. S1), while $\theta_2$ co-aligns with the angle of $[\bar{1}\,0\,\bar{1}]^*$ axis. This agrees with the results for the field range $2\text{ T} \leq \mu_0 H \leq 5$ T, shown in the main text. The same rotation of magnetic axes is also observed for $\mu_0 H = 1$ T (Fig. S2).

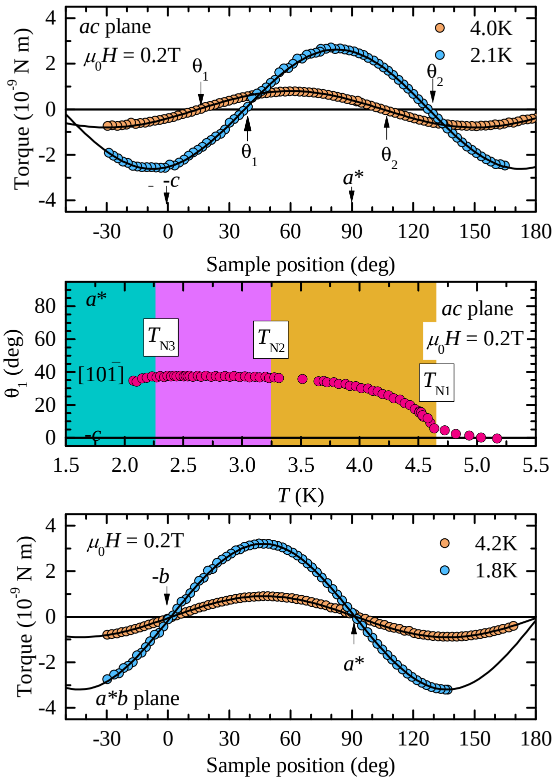


FIG. S1. Top panel: Angular dependence of torque measured in $\mu_0 H = 0.2$ T in the $ac$ plane at $T = 4.0$ K and 2.1 K. Middle panel: Temperature dependence of $\theta_1$ in the $ac$ plane. Transition temperatures are taken from previously published data [4]. Bottom panel: Angular dependence of torque measured in $\mu_0 H = 0.2$ T in the $a^*b$ plane at $T = 4.2$ K and 1.8 K. These results were used in previous publication [4]. Solid lines in top and bottom panel represent fits to Eqs. (1a) and (1b) from the main text.

In order to analyze the temperature-dependent curves obtained from the measured torque curves for $2\text{ T} \leq \mu_0 H \leq 5$ T, we first take a look at the temperature dependence of torque obtained previously in low magnetic field. In Fig. S3 we plot the temperature dependence

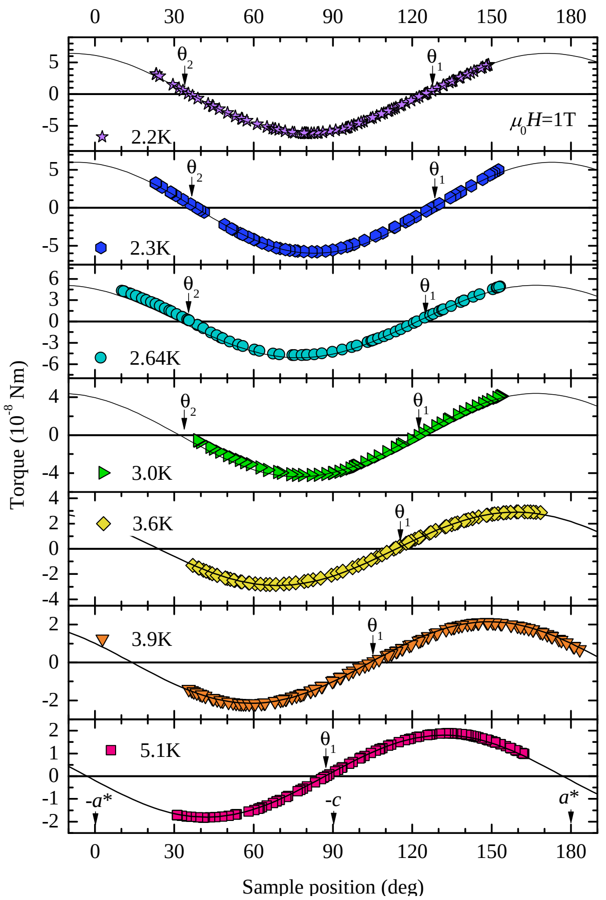


FIG. S2. Angular dependence of torque measured in $\mu_0 H = 1$ T in the *ac* plane. Solid lines represent Eq. (1a) from the main text. The uncertainty of the measured temperature of $\pm 0.1$ K is present due to the temperature lag which might be present between the calorimeter temperature (shown in figure) and the sample temperature.

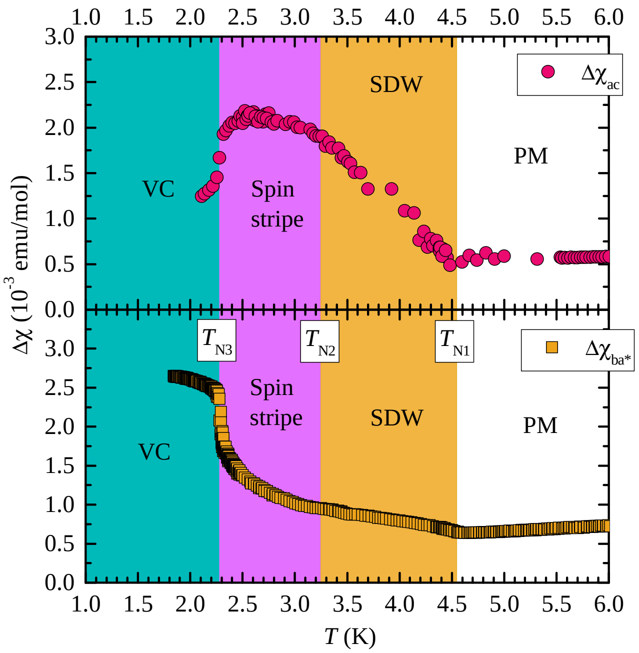


FIG. S3. Top: Temperature dependence on torque amplitude in the *ac* plane measured in $\mu_0 H = 0.2$ T. Bottom: Temperature dependence on torque amplitude in the $a^*b$ plane measured in $\mu_0 H = 0.2$ T. These results were used in previous publication [4].

of magnetic susceptibility anisotropy $\Delta\chi$, obtained from torque $\tau \propto \Delta\chi$ [Eqs. (1) in the main text]. In the *ac* plane (top panel of Fig. S3) the phase transition at $T_{N_1}$ is marked by a kink followed by a steep increase of the susceptibility anisotropy on further cooling. The phase transition to the spin-stripe phase at $T_{N_2}$ is not marked by any sharp feature, but rather by change to a much weaker, almost plateau-like, temperature dependence on cooling. The torque phase $\theta_1$ also stops changing when the system enters the spin-stripe phase, as can be seen in the middle panel of Fig. S1. Finally, the phase transition to the VC phase in the *ac* plane is observed by a sharp change (drop) of both the torque amplitude and the torque phase at $T_{N_3}$.

In the $a^*b$ plane the kink is also observed at $T_{N_1}$, and is followed by a weak increase of $\Delta\chi$ on cooling (bottom panel of Fig. S3). At $T_{N_2}$ an inflection point is observed followed by a steeper increase of anisotropy with decreasing temperature which almost diverges just before $T_{N_3}$ is reached. Finally, at $T_{N_3}$ a sharp kink is observed followed by a weak temperature dependence of $\Delta\chi$ on further cooling for $T < T_{N_3}$.

## ANISOTROPIC PHASE DIAGRAM

A full set of torque measurements for the *ac* plane is shown in Fig. S4, and for the $a^*b$ plane in Fig. S5. The results obtained from the macroscopic model presented in Sec. III B in the main text are plotted by solid lines in both figures. The anisotropic phase diagram represented in Fig. 6 in the main text was constructed using the procedure described below.

In Figs. S6 and S7 we show several chosen temperature and field-dependencies of torque obtained from the torque curves measured in the $a^*b$ and *ac* plane respectively (Figs. S4 and S5).

For both planes the phase transition to the VC phase at $T_{N_3}$ is easily observed (for angles at which it occurs) as a characteristic sharp change of torque amplitude (red dashed arrows in Figs. S6 and S7), similar to what is observed in low field, as discussed above. The error bar given in phase diagram in Fig. 6 of the main text represents the uncertainty of the reading which is limited by the temperature resolution of our experiment.

The phase transition to the spin-stripe phase at $T_{N_2}$ is harder to detect, especially for some field directions. Here we exploit the behavior observed in low magnetic

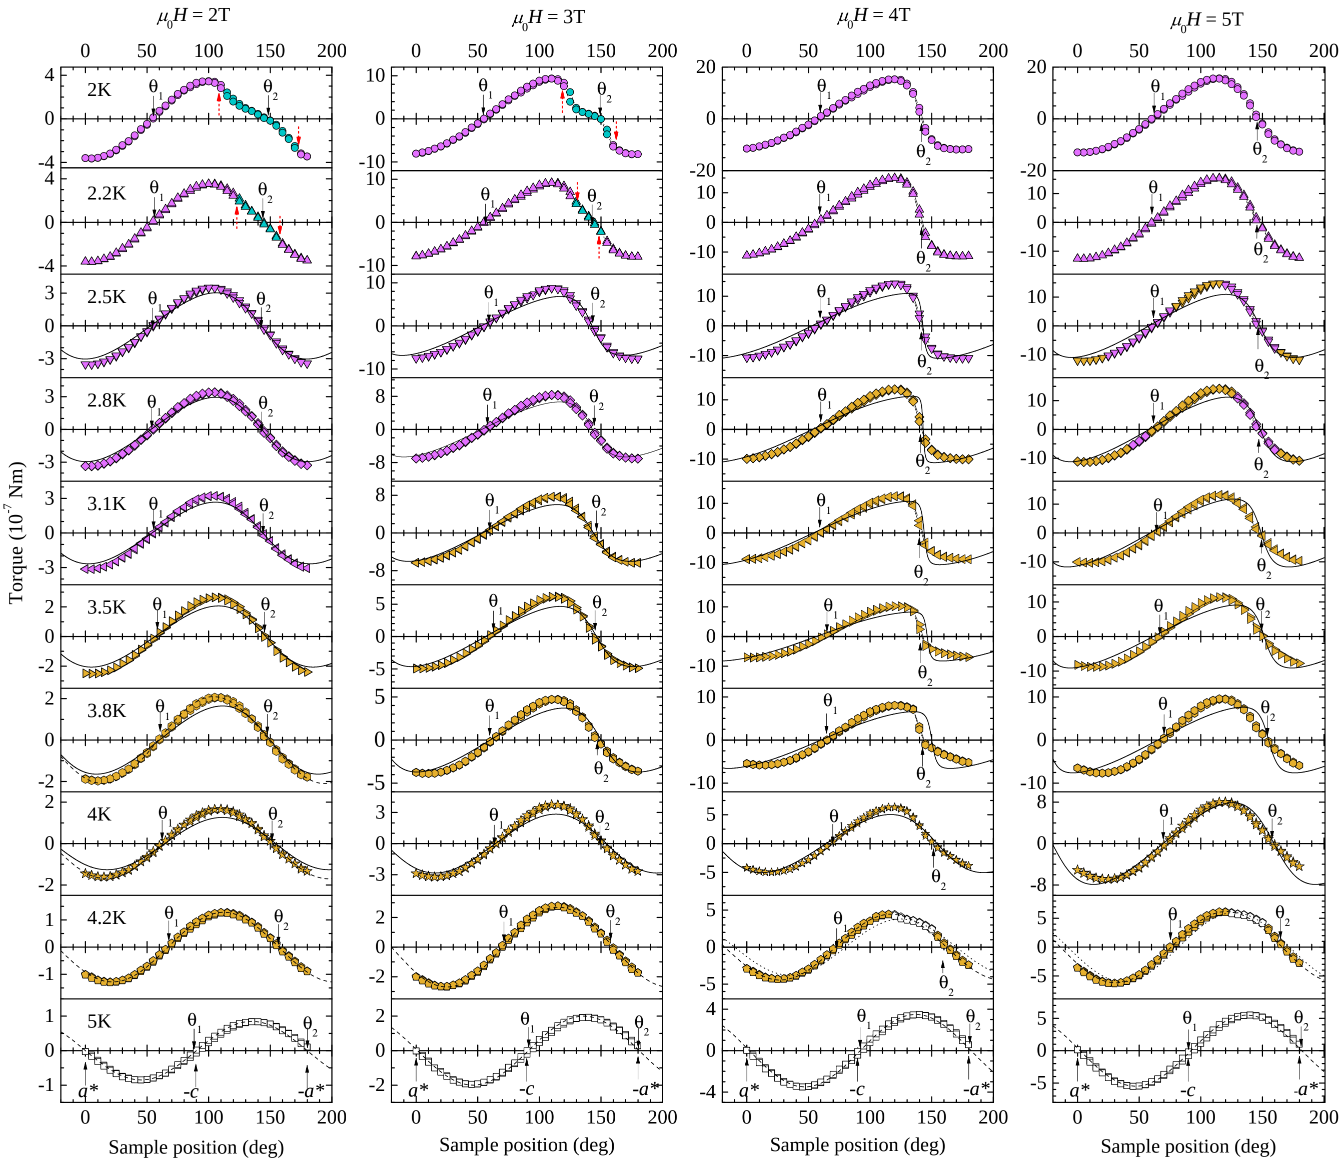


FIG. S4. Angular dependencies of torque in the $ac$ plane measured for chosen temperatures between $2 \leq T \leq 5$K in magnetic field $\mu_0 H = 2$, 3, 4 and 5 T. Black dashed lines represent Eq. (1b) while solid lines represent the torque obtained in case of a simple model of in-plane reorientation of spins (see Sec. III B in the main text). The dashed lines for $\mu_0 H > 2$ T were obtained by multiplying the line for $\mu_0 H = 2$ T by $H^2/2^2$ since, according to Eq. (1b) in the main text the torque is expected to have a $H^2$ dependence. Colors of data points represent different magnetic phases obtained from our analysis in Sec. III C of the main text: PM phase - white, SDW phase - gold, spin-stripe phase - magneta, VC phase - cyan. Solid black arrows denote $\theta_1$ and $\theta_2$ and dashed red arrows the phase boundary between the VC and the spin-stripe phases.

field, described in the previous section. For the $a^*b$ plane we observe an inflexion followed by a steep increase of torque magnitude which precludes the $T_{N_3}$. The estimated $T_{N_2}$ is shown by a black arrow in Fig. S6. In the $ac$ plane $T_{N_2}$ was attributed to the point where the torque amplitude starts to increase less rapidly with decreasing temperature, an effect observed for the low-field behavior. However, the estimated $T_{N_2}$, marked by black arrow in Fig. S7, has a large uncertainty, especially for $\mu_0 H = 4$ and 5 T. This uncertainty is displayed by error bars in Fig. 6 in the main text. A hysteresis observed for some angles is most likely an experimental artifact connected to the goniometer, since it is also observed for the same angles in curves measured at $T = 5$ K in the paramagnetic state.

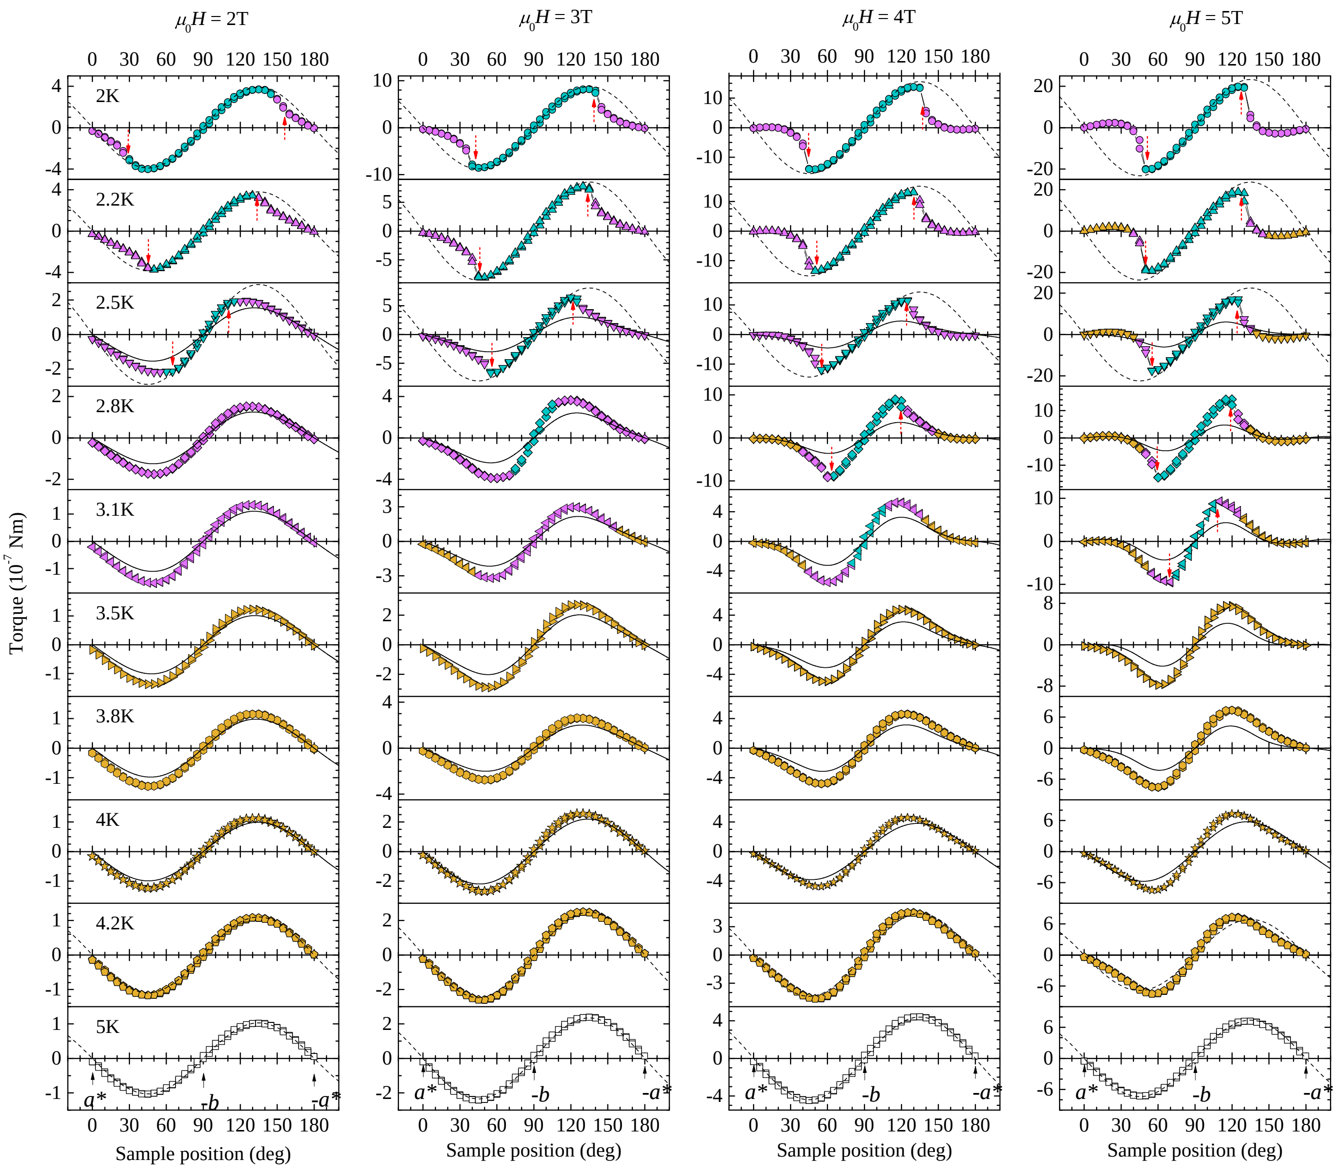


FIG. S5. Angular dependencies of torque in the $a^*b$ plane measured for chosen temperatures between $2 \leq T \leq 5$K in magnetic field $\mu_0 H = 2$, 3, 4 and 5 T. Black dashed lines represent Eq. (1a) while solid lines represent the torque obtained in case of a simple model of in-plane reorientation of spins (see Sec. III B). The dashed lines for $\mu_0 H > 2$ T were obtained by multiplying the line for $\mu_0 H = 2$ T by $H^2/2^2$ since, according to Eq. (1a) the torque is expected to have a $H^2$ dependence. Colors of data points represent different magnetic phases obtained from our analysis in Sec. III C of the main text: PM phase - white, SDW phase - gold, spin-stripe phase - magneta, VC phase - cyan. The red dashed arrows denote the phase transition boundary between the VC and the spin-stripe phase.

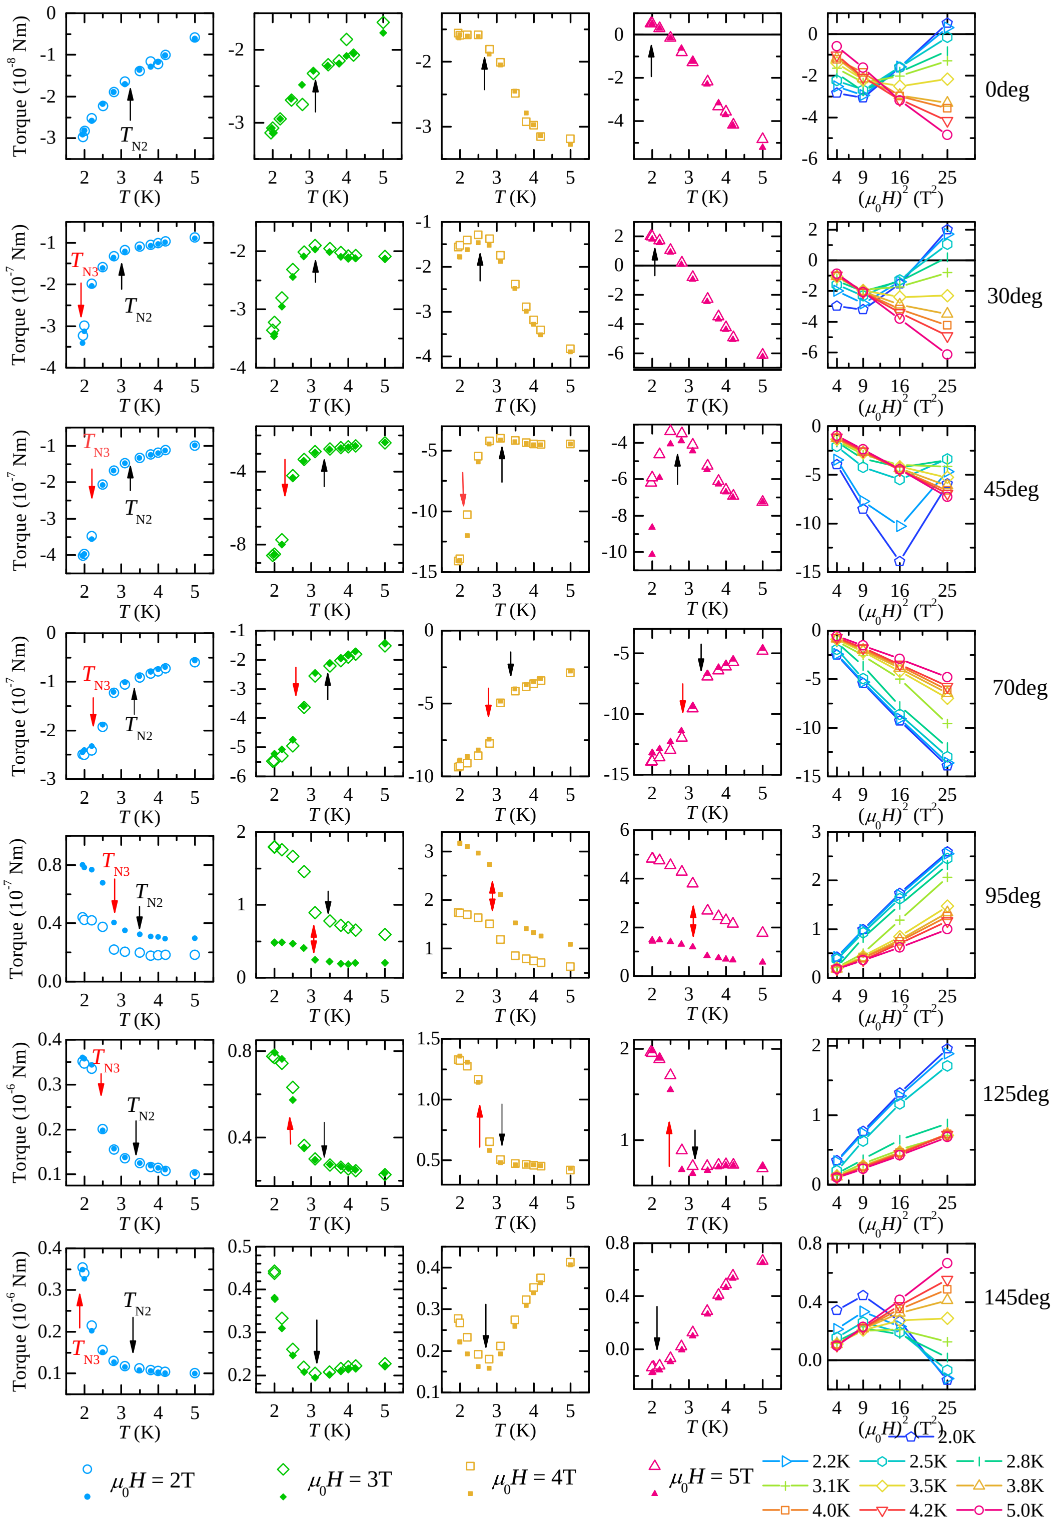


FIG. S6. From left to right: temperature dependence of torque measured in $\mu_0 H = 2$ (blue circles), 3 (green diamonds), 4 (yellow squares) and 5 T (pink triangles) and field dependence measured at different temperatures for the several chosen sample positions in the $a^*b$ plane. Black arrow points to $T_{N_2}$ phase transition and red arrow to $T_{N_3}$. Data points were obtained from torque curves show in Fig. S5. Empty and solid symbols denote the data obtained, respectively, from torque curves recorded while rotating the sample from 0° to 180° and back. In the figures showing the field dependence (panels on the right) only the points from the positive rotation curves are shown for clarity. Field dependence demonstrates the deviation from Eq. (1b) in the main text which predicts $\tau \propto H^2$.

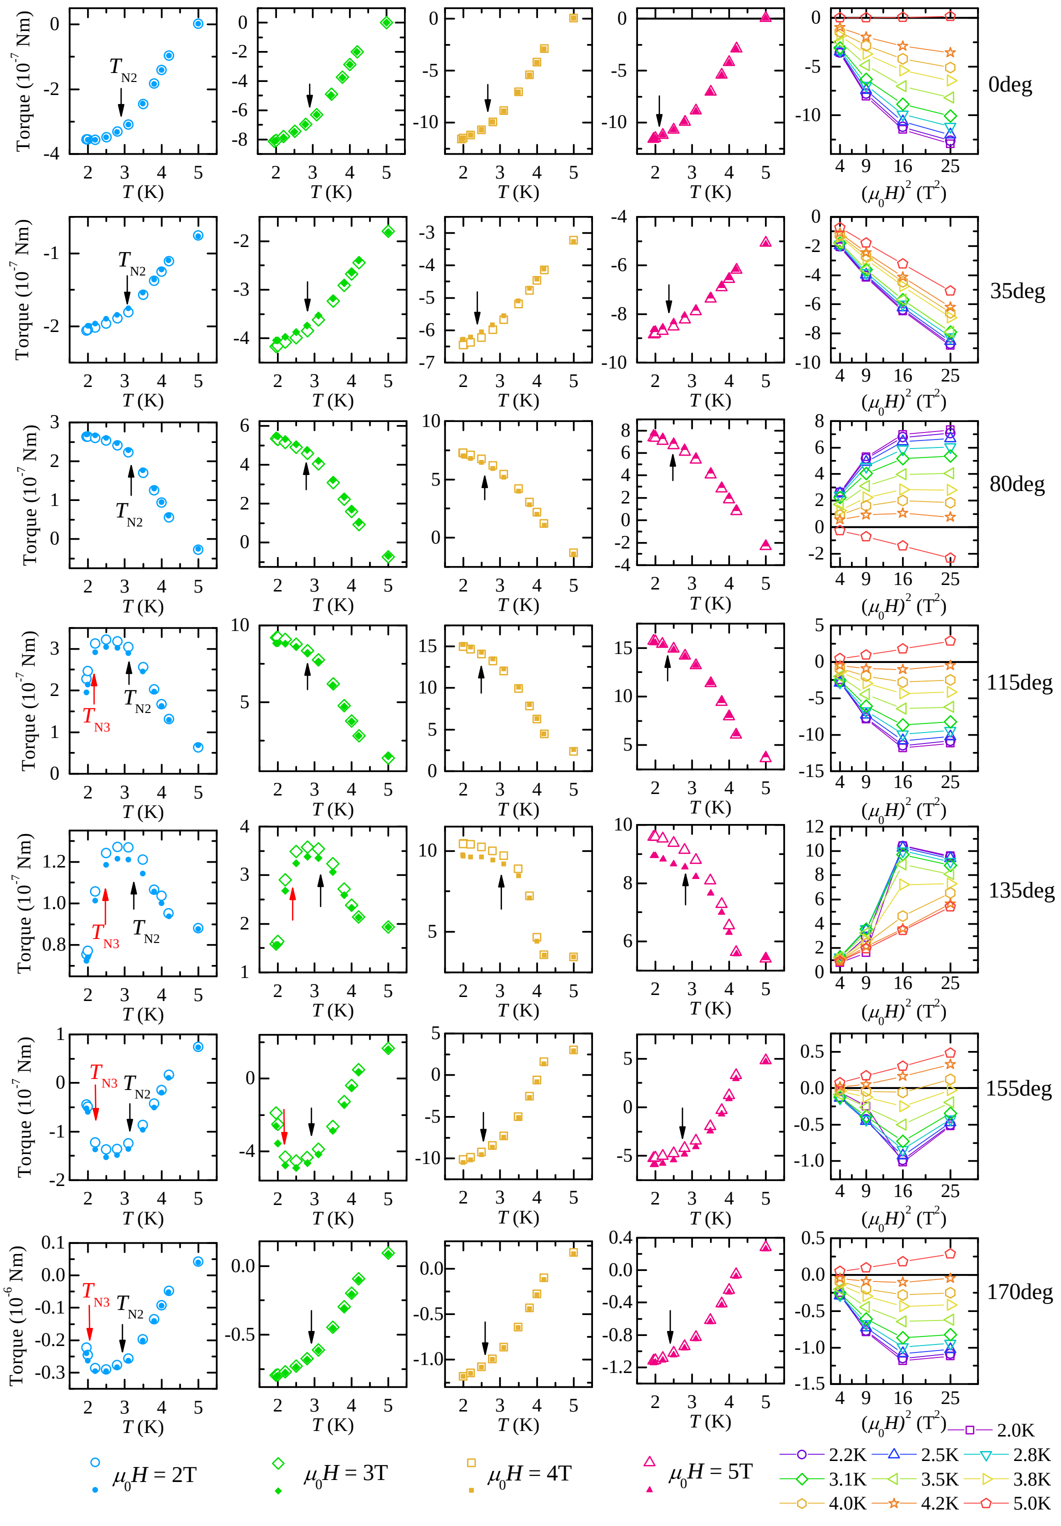


FIG. S7. From left to right: temperature dependence of torque measured in $\mu_0 H = 2$ (blue circles), 3 (green diamonds), 4 (yellow squares) and 5 T (pink triangles) and field dependence measured at different temperatures for the several chosen sample positions in the $ac$ plane. Black arrow points to $T_{N_2}$ phase transition and red arrow to $T_{N_3}$. Data points were obtained from torque curves show in Fig. S4. Empty and solid symbols denote the data obtained, respectively, from torque curves recorded while rotating the sample from 0° to 180° and back. In the figures showing the field dependence (panels on the right) only the points from positive rotation curves are shown for clarity. Field dependence demonstrates the deviation from Eq. (1a) in the main text which predicts $\tau \propto H^2$.

## SPIN REORIENTATION

The spin-axis reorientation obtained from Eq. (2) in the main text, which accompanies the calculated torque curves show in Figs. 2 and 3 of the main text, is shown in Figs. S8 and S9 for the $ac$ and $a^*b$ plane, respectively.

For each temperature and applied magnetic field, the maximal rotation of the spin axis has different value. Only for fields of 4 and 5 T which are larger than the spin-flop field the maximal rotation amounts to 90°. The maximal spin axis rotation is introduced as a color scale in the phase diagram given in Fig. 6 in the main text. The apparent discontinuity which appears for some temperatures in $\mu_0 H = 4$ T and 5 T does not in fact represent a sharp jump in $\theta_0$, which we emphasize by plotting the equivalent solution $\theta_0 + 180°$ by the dashed lines in Fig. S8.

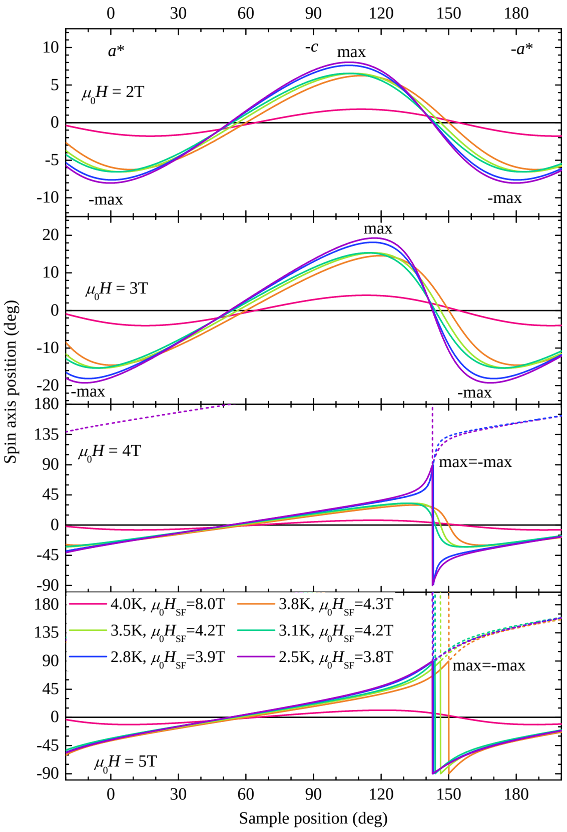


FIG. S8. Calculated spin axis position in the $ac$ plane with respect to the easy axis position using Eq. (2) in Sec. III B of the main text. Sample position denotes the orientation of the magnetic field with respect to the crystal axes. Angles denoting the field directions $a^*$, $-c$ and $-a^*$ are labeled in the top panel. Positive value of the spin axis position denotes rotation from the easy axis direction towards the $a^*$ direction ($+b$ rotation), and negative towards the $c$ axis ($-b$ direction). Dashed lines represent the equivalent solution $\theta_0 + 180°$.

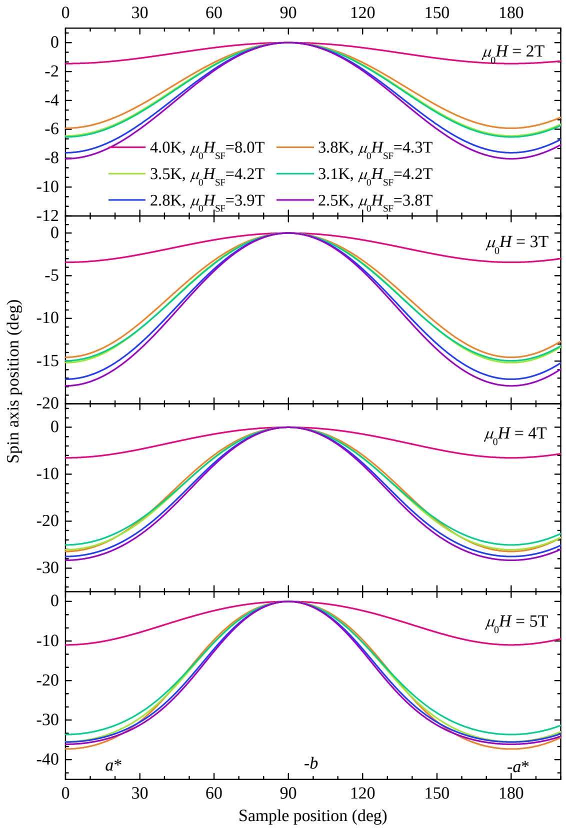


FIG. S9. Calculated spin axis position in the $a^*b$ plane with respect to the easy axis position using Eq. (2) in Sec. III B of the main text. Sample position denotes the orientation of the magnetic field with respect to the crystal axes. Angles denoting the field directions $a^*$, $-b$ and $-a^*$ are labeled in the bottom panel. The rotation of the spin axis is negative and it denotes a rotation towards the $c$ axis.

* mirta@ifs.hr


[1] Y. O. Savina, O. M. Bludov, V. A. Pashchenko, S. L. Gnatchenko, P. Lemmens, and H. Berger, Low Temperature Physics **41**, 283 (2015).

[2] F. Weickert, N. Harrison, B. L. Scott, M. Jaime, A. Leitmae, I. Heinmaa, R. Stern, O. Janson, H. Berger, H. Rosner, and A. A. Tsirlin, Phys. Rev. B **94**, 064403 (2016).

[3] M. Pregelj, A. Zorko, M. Klanjšek, O. Zaharko, J. S. White, O. Prokhnenko, M. Bartkowiak, H. Nojiri, H. Berger, and D. Arčon, Phys. Rev. B **100**, 094433 (2019).

[4] M. Pregelj, O. Zaharko, M. Herak, M. Gomilšek, A. Zorko, L. C. Chapon, F. Bourdarot, H. Berger, and D. Arčon, Phys. Rev. B **94**, 081114 (2016).
